# Supplementary material for: Simple, Fast, and Scalable Reachability Oracle
Source: arXiv:1305.0502 source file (2013-07-01)
Supplement: Supplementary file 1 [file appendix.tex]

\vspace*{-2.0ex}
\appendix

\comment{
\section{Proof of Lemma 1.}
\bproof
First, we prove $E^\ast \subseteq TC(V^\ast)$ by way of contradiction. 
Assuming $E^\ast$ contains edge $(u,v) \notin TC(V^\ast)$, i.e., $u$ cannot reach $v$ in the original graph $G$. 
Since $u$ and $v$ are both backbone vertices, then for the unreachable pair $(u,v)$, we can find $u^\ast=u$ and $v^\ast=v$, such that $u^\ast$ reaches $v^\ast$. This clearly contradicts the definition of reachability backbone. 

Second, if the original backbone edge set $TC^\ast(V^\ast) \subseteq E^\ast$, then, based on the definition of {\em transitive reduction}, all the reachability information in $G^\ast=(V^\ast,E^\ast)$ is equivalent to ${\bf G^\ast}=(V^\ast,TC^\ast(V^\ast))$. In other words, they have the same transitive closure. Then, clearly ${\bf G^\ast}=(V^\ast,TC^\ast(V^\ast))$ is also a  reachability backbone of $G$. 
If the original backbone edge set $E^\ast \subset TC^\ast(V^\ast)$, clearly, for any non-local pair $(u,v)$ in graph $G$, if there exist two vertices $u^\ast$ and $v^\ast$ in $V^\ast$, such that $(u,u^\ast)$ and $(v^\ast,v)$ are both local pairs in $G$ and $u^\ast$ can reach $v^\ast$ in $G^\ast$; then, $u^\ast$ can reach $v^\ast$ in ${\bf G^\ast}=(V^\ast,TC^\ast(V^\ast)$. 
For any unreachable pair $(u,v)$ in $G$, we need show that there does not exist two vertices $u^\ast$ and $v^\ast$ in $V^\ast$, such that $(u,u^\ast)$ and $(v^\ast,v)$ are both local pairs in $G$ and $u^\ast$ can reach $v^\ast$ in ${\bf G^\ast}=(V^\ast,TC^\ast(V^\ast)$. 
Again we can prove this by way of contradiction. Since if there exists $u^\ast$ and $v^\ast$ in $V^\ast$, such that $(u,u^\ast)$ and $(v^\ast,v)$ are both local pairs in $G$ and $u^\ast$ can reach $v^\ast$ in ${\bf G^\ast}=(V^\ast,TC^\ast(V^\ast)$, then, $u$ can reach $v$ in the original graph (as $TC(V^\ast)$ is the transitive closure on $V^\ast$ in the original graph $G$). This contradicts to the assumption that $(u,v)$ is unreachable pair in $G$. 
Put these together, ${\bf G^\ast}=(V^\ast,TC^\ast(V^\ast))$ is always a  reachability backbone of $G$. 
\eproof
}

\section{Proof of Theorem 1.}
\bproof 
We reduce the classical NP-hard problem, set-cover problem (SCP), to this problem
In \rw{the classical set-cover problem}{SCP}, let $\mathcal{U}$ be the ground set and $\mathcal{C}$ records all the candidate sets, where for any candidate set $C \in \mathcal{C}$ and $C \subseteq \mathcal{U}$. 
The goal is to determine whether there are $K$ (or less ) candidate sets in $\mathcal{C}$ such that $\cup_i C_i = \mathcal{U}$. 
Now we\x{ show that how we can} transform it to the decision version of MRBVS discovery problem, i.e., 
whether there is a backbone vertex set containing $K$ or less vertices.  

We construct the following DAG based on a set cover instance: 
let $G=(X \cup Y \cup Z, E_{XY} \cup E_{YZ})$ be the DAG, where each vertex in $X$ and $Z$ corresponds \rw{}{to} a unique element in the ground set $\mathcal{U}$, and each element in $Y$ corresponds \rw{}{to} a candidate set in $\mathcal{C}$;  
the edge set $E_{XY}$ contains all the edges $(x_u,y_C)$ where $x_u$ is the corresponding vertices of element $u \in \mathcal{U}$ in the vertex set $X$, and $y_C$ is the corresponding vertex of candidate set $C \in \mathcal{C}$ in $Y$, and the element $u \in \mathcal{U}$ belongs to the  candidate set $C$ in $\mathcal{C}$; 
the edge set $E_{YZ} = Y \times Z$, i.e., it contains the edge set which connects any pair from a vertex in $Y$ to a vertex in $Z$. 

Given this, we will show that for the locality parameter $\epsilon=1$, the minimal reachability backbone vertex set (MRBVS) contains only vertices in $Y$ and directly corresponds to the minimal set cover solution. 
Thus, the set cover problem which asks whether there is a  $K$ or less vertex cover can be directly answered by the solution on whether there is a $K$ or less backbone vertex set in the above problem instance. 

For the first claim (MRBVS contains only vertices in $Y$), if it is not, let the minimal reachability backbone vertex set $V^\ast=X^\prime \cup Y^\prime \cup Z^\prime$, where $X^\prime$,$Y^\prime$, and $Z^\prime$ contains the backbone vertices from vertex set $X$, $Y$, and $Z$, respectively. 

\noindent{\bf Case 1 ($\boldsymbol{X^\prime\neq \emptyset}$ and $\boldsymbol{Z^\prime = \emptyset}$): } In this case, we can simply drop all the vertices in $X^\prime$, and $V^\ast=Z^\prime$ is enough to serve as the backbone vertices. 
This is because for any non-local pair $(x,z)$, there exist $x^\ast$ and $y^\ast$ where $y^\ast$ must be in $Y^\prime$, and either (1) $x^\ast=x$ in $X^\prime$ or (2) $x^\ast=y^\ast$ in $Y^\prime$. For (1), we must have $(x,y^\ast) \in E_{XY}$ and thus we can always replace $x^\ast$ with $y^\ast$. Basically, $Y^\prime$ would contain enough backbone vertices.  A similar proof holds for {\bf $\boldsymbol{X^\prime=\emptyset}$ and $\boldsymbol{Z^\prime \neq \emptyset}$}. 

\noindent{\bf Case 2 ($\boldsymbol{X^\prime \neq \emptyset}$ and $\boldsymbol{Z^\prime \neq \emptyset}$):} 
In this case, we construct $Y_s$ as follows: each vertex $x \in  X^\prime$ randomly chooses an edge $(x,y)$ in $E_{XY}$ and adds $(x,y)$ into $Y_s$. It is easy to see that $|Y_s| \leq |X^\prime$. 
We claim the following backbone vertex set $Y^\prime \cup Y_s$ is enough to recover the reachability between any  non-local pair in $G$. 
This is because for any non-local pair $(x,z)$, which needs $x^\ast=x$ and $z^\ast=z$ in the original backbone vertex set, it now can use $y \in Y_s$ ($(x,y) \in E_{XY}$) to serve as the backbone vertices: $x^\ast=y$ and $z^\ast=y$. 
Since $|Y_s \cup Y^\prime| < |X^\prime \cup Y^\prime \cup Z^\prime|$, this is clearly impossible due to the minimality assumption. 
To sum, the minimal reachability backbone vertex set $V^\ast$ should contain only the vertices in $Y$. 

Now, we show that $V^\ast$ directly corresponds to the solution of the minimal \rw{the original set cover problem}{SCP}. 
By way of contradiction, if the corresponding set of candidates in $V^\ast$ is not the minimal one which can cover the ground set $\mathcal{U}$, and then we claim $V^\prime$ which corresponds to the minimal set cover is also a backbone vertex set. This is because for any non-local pair $(x,z)$, there must exist $y$ in $V^\prime$ where $(x,y) \in E_{XY}$ since $x$ in the ground set is covered by some candidate $C$ (corresponding to $y$). Clearly, this contradicts our assumption that $V^\ast$ is the minimal one. 
\eproof

\section{Proof of Lemma 3.}
%~\ref{NPhardness}
\bproof
Since $(u,v) \in E^\ast$ only if $(u,v)$ is local pair in $G$ ($u\rightarrow v$), therefore, $E^\ast \subseteq TC(V^\ast)$. 
Now, we show $TC^\ast(V^\ast) \subseteq E^\ast$, i.e.,  if $u \rightarrow v$ in $G$, the $u\rightarrow v$ in $G^*$=($V^*$,$E^*$).
If $d(u,v) \leq\epsilon$, then $u\rightarrow v$ in $G^*$=($V^*$,$E^*$) by definition.
If $d(u,v)=\epsilon+1$, then based on Lemma 2, there exists a $x\in V^*$ such that $d(u,x)\leq\epsilon$ and $d(x,v)\leq\epsilon$.
So, based on the definition of $G^*$, $u\rightarrow v$. Now, if $d(u,v)>\epsilon+1$, then there is a vertex $w$ such that $d(u,w)=\epsilon+1$ and $w\rightarrow v$.
Based on Lemma 2, we can find a vertex $x\in V^*$ such that $d(u,x)\leq\epsilon$ and $d(x,w)\leq\epsilon$.
So, the proof is reduced to $d(x,v)$. We apply the same procedure until we reach a vertex $y\in V^*$ with $d(y,v)\leq\epsilon$.
Then, based on the definition of $G^*$, $u\rightarrow v$.
\eproof
